# Supplementary material for: Simultaneous Perturbation Algorithms for Batch Off-Policy Search
Source: arXiv:1403.4514 source file (2014-03-31)
Supplement: Supplementary file 1 [file Appendix_finitetimeanalysis.tex]

to be done..
